# Supplementary material for: Data Consistency in Transactional Storage Systems: a Centralised Approach
Source: arXiv:1901.10615 source file (2019-10-04)
Supplement: Supplementary file 1 [file counter-example-si-not-cp-ua.tex]

\subsection{\( \SI \) is not intersection of \( \CP \) and \( \UA \) on dependency graph}
\label{sec:si-not-intersect-cp-ua}
We refer reader to \cref{sec:dependent-graph,sec:abstract-execution} for the full details of dependency graphs and abstract execution.
Here we show why when on abstract executions, the definition of \( \SI \) is intersection of \( \CP \) and \( \UA \), but it is not the case on the definition on dependency graphs.
Let consider the following dependency graph which is allowed by both \( \CP \) and \( \UA \):

\begin{center}
\begin{tikzpicture}[scale=0.85, every node/.style={transform shape}]

% t0
\draw pic {transaction={t0}{%
        $\otW$/$\key_1$/$1$%
        , $\otW$/$\key_2$/$1$%
}};
\path(t0.west)  node[anchor=east] (t0lbl) {$\txid_0$};
% t1
\draw pic at ($(t0.east) + (2,0.2)$) {transaction={t1}{%
        $\otW$/$\key_1$/$2$%
        , $\otR$/$\key_4$/$0$%
}};
\path(t1.east) node[anchor=west] (t1lbl) {$\txid_1$};
% t2
\draw pic at ($(t0.south) + (-0.8,-1)$)  {transaction={t2}{%
        $\otW$/$\key_3$/$4$%
        , $\otR$/$\key_2$/$0$%
}};
\path(t2.west) node[anchor=east] (t2lbl) {$\txid_2$};
% t3
\draw pic at ($(t1.south) + (-0.8,-1)$) {transaction={t3}{%
        $\otW$/$\key_3$/$3$%
        , $\otW$/$\key_4$/$1$%
}};
\path(t3.east) node[anchor=west] (t3lbl) {$\txid_3$};

\path[->]
(t0.north) edge[bend left=30] node[above, yshift=3pt, xshift=0pt, pos=0.5] {$\WW$} (t1.north)
(t2.north) edge[bend left=30] node[below, yshift=0pt, xshift=-20pt, pos=0.7] {$\RW$} (t0.south)
(t1.south) edge[bend left=30] node[above, yshift=0pt, xshift=20pt, pos=0.6] {$\RW$} (t3.north)
(t3.south) edge[bend left=30] node[below, yshift=-3pt, xshift=0pt, pos=0.5] {$\WW$} (t2.south);

\end{tikzpicture}
\end{center}

Now we convert the graph to abstract executions.
First we can only choose one of the following arbitration relations:
\(
    \txid_0 \toEDGE{\AR} \txid_1 \toEDGE{\AR} \txid_2 \toEDGE{\AR} \txid_3
\)
or 
\(
    \txid_3 \toEDGE{\AR} \txid_2 \toEDGE{\AR} \txid_0 \toEDGE{\AR} \txid_1
\)
Such two relations guarantee the abstract executions converted from the dependency graph satisfy \( \SI \).
Then \( \UA \) requires \( \WW \in \VIS \), which means we might have the following abstract execution (the another one is symmetric):
\begin{center}
{
\begin{tikzpicture}[scale=0.85, every node/.style={transform shape}]

% t0
\draw pic {transaction={t0}{%
        $\otW$/$\key_1$/$1$%
        , $\otW$/$\key_2$/$1$%
}};
\path(t0.west)  node[anchor=east] (t0lbl) {$\txid_0$};
% t1
\draw pic at ($(t0.east) + (2,0.2)$) {transaction={t1}{%
        $\otW$/$\key_1$/$2$%
        , $\otR$/$\key_4$/$0$%
}};
\path(t1.east) node[anchor=west] (t1lbl) {$\txid_1$};
% t2
\draw pic at ($(t0.south) + (-0.8,-1)$)  {transaction={t2}{%
        $\otW$/$\key_3$/$4$%
        , $\otR$/$\key_2$/$0$%
}};
\path(t2.west) node[anchor=east] (t2lbl) {$\txid_2$};
% t3
\draw pic at ($(t1.south) + (-0.8,-1)$) {transaction={t3}{%
        $\otW$/$\key_3$/$3$%
        , $\otW$/$\key_4$/$1$%
}};
\path(t3.east) node[anchor=west] (t3lbl) {$\txid_3$};

\path[->]
(t0.north) edge[bend left=30] node[above, yshift=3pt, xshift=0pt, pos=0.5] {$\AR,\VIS$} (t1.north)
(t1.south) edge[bend left=30] node[above, yshift=0pt, xshift=20pt, pos=0.6] {$\AR$} (t3.north)
(t3.south) edge[bend left=30] node[below, yshift=-3pt, xshift=0pt, pos=0.5] {$\AR,\VIS$} (t2.south);
\end{tikzpicture}
}%
\end{center}
By the constrain \( \AR ; \VIS \subseteq \VIS \), which should be satisfies by both \( \CP \) and especially \( \SI \)  on abstract execution, we have the following abstract execution:
\begin{center}
{
\begin{tikzpicture}[scale=0.85, every node/.style={transform shape}]

% t0
\draw pic {transaction={t0}{%
        $\otW$/$\key_1$/$1$%
        , $\otW$/$\key_2$/$1$%
}};
\path(t0.west)  node[anchor=east] (t0lbl) {$\txid_0$};
% t1
\draw pic at ($(t0.east) + (2,0.2)$) {transaction={t1}{%
        $\otW$/$\key_1$/$2$%
        , $\otR$/$\key_4$/$0$%
}};
\path(t1.east) node[anchor=west] (t1lbl) {$\txid_1$};
% t2
\draw pic at ($(t0.south) + (-0.8,-1)$)  {transaction={t2}{%
        $\otW$/$\key_3$/$4$%
        , $\otR$/$\key_2$/$0$%
}};
\path(t2.west) node[anchor=east] (t2lbl) {$\txid_2$};
% t3
\draw pic at ($(t1.south) + (-0.8,-1)$) {transaction={t3}{%
        $\otW$/$\key_3$/$3$%
        , $\otW$/$\key_4$/$1$%
}};
\path(t3.east) node[anchor=west] (t3lbl) {$\txid_3$};

\path[->]
(t0.north) edge[bend left=30] node[above, yshift=3pt, xshift=0pt, pos=0.5] {$\AR,\VIS$} (t1.north)
(t0.south) edge[bend right=30] node[below, yshift=0pt, xshift=-20pt, pos=0.3] {$\VIS$} (t2.north)
(t1.south) edge[bend left=30] node[above, yshift=0pt, xshift=20pt, pos=0.6] {$\AR$} (t3.north)
(t3.south) edge[bend left=30] node[below, yshift=-3pt, xshift=0pt, pos=0.5] {$\AR,\VIS$} (t2.south);
\end{tikzpicture}
}
\end{center}
This leads to contradiction:
\( \txid_2 \) should see \( \txid_0 \) but \( \txid_2 \) did not read the value 1 for \( \key_2 \) written by \( \txid_0 \).
